# Supplementary material for: Defense against Backdoor Attacks via Identifying and Purifying Bad Neurons
Source: arXiv:2208.06537 source file (2022-08-13)
Supplement: Supplementary file 1 [file appendix.tex]

\section{Attack implementation details}
We summarize the implementation details of six backdoor attacks used in this paper as follows:
\begin{itemize}
    \item \textbf{BadNet:} A 3$\times$3 trigger with random pixel values is pasted in the top left corner of 5$\%$ training images, and labels tamper with 0.
    \item \textbf{Blend Attack:} We used the same trigger, a hello kitty image, in the original paper, blend ratio of 0.2, and inject rate of 0.05.
    \item \textbf{Enhanced Trigger Attack:} Following the original paper, we adopt the same random spatial transformation layer consisting of rotation and scale to pre-process the poison data. The associated parameters of the trigger used in this attack are identical to BadNet.
    \item \textbf{Invisible Attack:} We generated the same trigger with $32 \times 32$ resolution in the original paper and injection rate of 0.05.
    \item \textbf{Sinusoidal signal attack:} We used the backdoor trigger generation function in the original paper with $\delta=20$ and $f=6$ and injection rate of 0.1.
    \item \textbf{TrojanNN:} Based on the implementation of the original paper, we utilized the same reverse engineer technology to craft a $3 \times 3$ square trigger from the fully connected layer. Other parameters are set the same in BadNet.
\end{itemize}

\begin{table*}[t]
\begin{tabular}{@{}c|cc|cc|cc|cc|cc|cc@{}}
\toprule
Attack & \multicolumn{2}{c|}{BadNet} & \multicolumn{2}{c|}{BA} & \multicolumn{2}{c|}{ETA} & \multicolumn{2}{c|}{IA} & \multicolumn{2}{c|}{SIG} & \multicolumn{2}{c}{TrojanNN} \\ \midrule
Method & ACC & ASR & ACC & ASR & ACC & ASR & ACC & ASR & ACC & ASR & ACC & ASR \\ \midrule
before & 94.68 & 100.00 & 94.62 & 100.00 & 94.59 & 99.98 & 94.68 & 100.00 & 94.38 & 96.97 & 94.71 & 100.00 \\
Pruning + AM & 93.17 & 69.57 & 92.29 & 79.65 & 93.41 & 68.52 & 94.53 & 87.53 & 93.16 & 38.53 & 92.31 & 97.82 \\
Pruning + BS & 93.58 & 17.58 & 93.01 & 19.25 & 93.58 & 24.92 & 93.07 & 13.78 & 93.52 & 12.84 & 93.41 & 20.88 \\
Purifying + AM & 93.70 & 34.06 & 93.91 & 29.32 & 93.56 & 45.50 & \textbf{94.57} & 35.19 & 93.64 & 27.10 & 93.84 & 63.08 \\
Purifying + BS & \textbf{94.14} & \textbf{0.49} & \textbf{94.09} & \textbf{2.87} & \textbf{94.11} & \textbf{4.94} & 94.23 & \textbf{9.48} & \textbf{93.69} & \textbf{1.48} & \textbf{94.52} & \textbf{2.41} \\ \bottomrule
\end{tabular}
\caption{Comparison of backdoor defense with different purifying strategies and neuron importance evaluation metrics on SVHN.}
\label{table_importance_comp_svhn}
\end{table*}

\begin{table*}[t]
\begin{tabular}{@{}c|cc|cc|cc|cc|cc|cc@{}}
\toprule
Attack & \multicolumn{2}{c|}{BadNet} & \multicolumn{2}{c|}{BA} & \multicolumn{2}{c|}{ETA} & \multicolumn{2}{c|}{IA} & \multicolumn{2}{c|}{SIG} & \multicolumn{2}{c}{TrojanNN} \\ \midrule
Method & ACC & ASR & ACC & ASR & ACC & ASR & ACC & ASR & ACC & ASR & ACC & ASR \\ \midrule
before & 69.66 & 99.83 & 68.68 & 99.81 & 68.98 & 98.43 & 69.12 & 99.88 & 68.92 & 90.21 & 70.84 & 94.66 \\
Pruning + AM & 63.48 & 25.53 & 63.08 & 26.68 & 62.89 & 37.63 & 60.97 & 23.30 & 61.43 & 28.07 & 61.45 & 78.99 \\
Pruning + BS & 63.55 & 16.69 & 63.02 & 19.87 & 61.73 & 18.07 & 61.02 & 11.77 & 62.21 & 15.28 & 61.96 & 29.63 \\
Purifying + AM & 63.62 & 20.31 & 63.15 & 23.51 & \textbf{63.01} & 25.04 & 61.75 & 19.27 & 62.52 & 22.67 & 62.83 & 70.57 \\
Purifying + BS & \textbf{63.71} & \textbf{1.12} & \textbf{63.21} & \textbf{0.80} & 62.35 & \textbf{0.83} & \textbf{62.11} & \textbf{0.55} & \textbf{63.89} & \textbf{0.26} & \textbf{63.92} & \textbf{0.20} \\ \bottomrule
\end{tabular}
\caption{Comparison of backdoor defense with different purifying strategies and neuron importance evaluation metrics on CIFAR100.}
\label{table_importance_comp_cifar100}
\end{table*}

\section{Defense implementation details}
We list the detailed defense settings of Fine-Pruning, Fine-tuning, KD, and NAD for reference:
\begin{itemize}
    \item \textbf{Fine-Pruning:} As suggested in the original paper, we pruned the last layer of the model with a pruning rate of 0.1, where AM is measured over a random subset of the training set as same to BS.
    \item \textbf{Fine-tuning:} Following the original paper, we adopted a standard fine-tuning procedure with a fixed learning rate of 0.1, momentum factor of 0.9, $L_2$ weight decay factor of $1 \times 10^{-4}$, and cross-entropy loss function to recover the backdoored model.
    \item \textbf{KD:} The standard knowledge approach is employed to recover the backdoored model, where cross-entropy loss and KL divergence are fused together as the overall loss function.
    The weights of the two loss terms are set to 0.5 along with the temperature of 2 and epoch of 50.
    \item \textbf{NAD:} We replicated the defense of NAD, where the backdoored model is fine-tuned for 10 epochs with an initial learning rate of 0.1 and a momentum of 0.9.
    The learning rate is divided by 10 after every 2 epochs.
\end{itemize}

\begin{figure*}[!h]
\centering
\begin{subfigure}{0.15\textwidth}
\centering
    \includegraphics[width=0.99\linewidth]{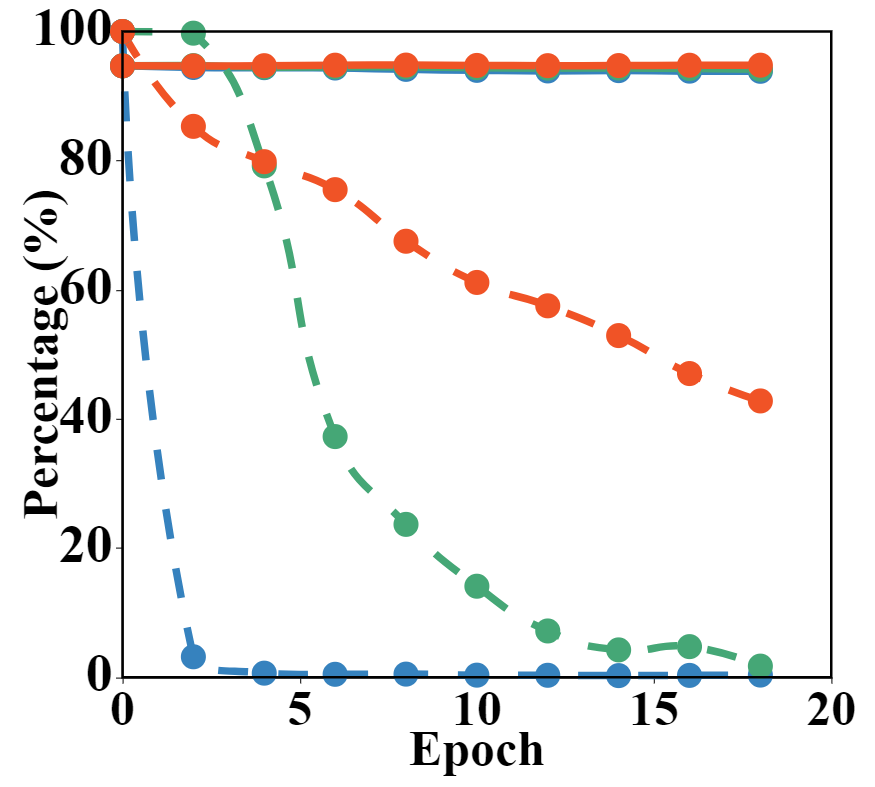}
    \caption{BadNet}
\end{subfigure}%
\begin{subfigure}{0.15\textwidth}
\centering
    \includegraphics[width=0.99\linewidth]{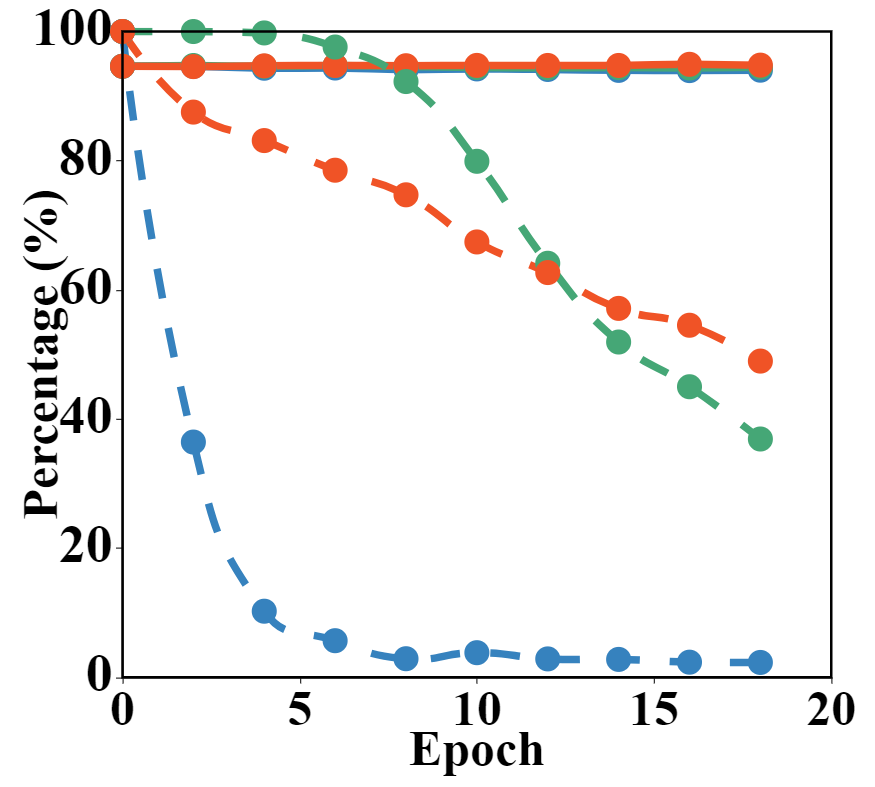}
    \caption{BA}
\end{subfigure}
\begin{subfigure}{0.15\textwidth}
\centering
    \includegraphics[width=0.99\linewidth]{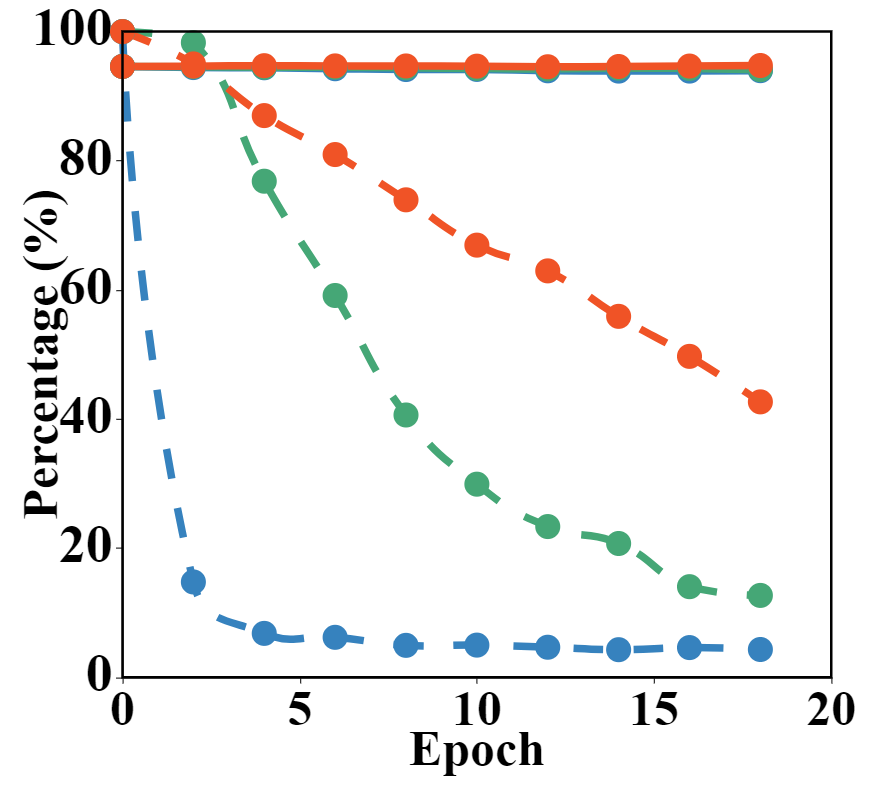}
    \caption{ETA}
\end{subfigure}
\begin{subfigure}{0.15\textwidth}
\centering
    \includegraphics[width=0.99\linewidth]{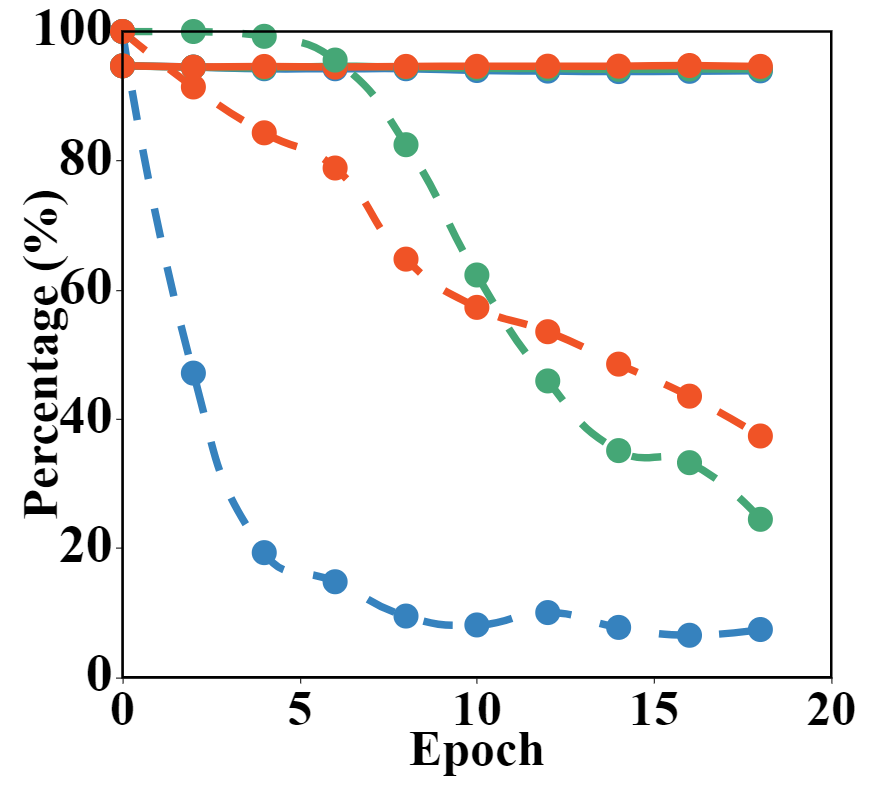}
    \caption{IA}
\end{subfigure}
\begin{subfigure}{0.15\textwidth}
\centering
    \includegraphics[width=0.99\linewidth]{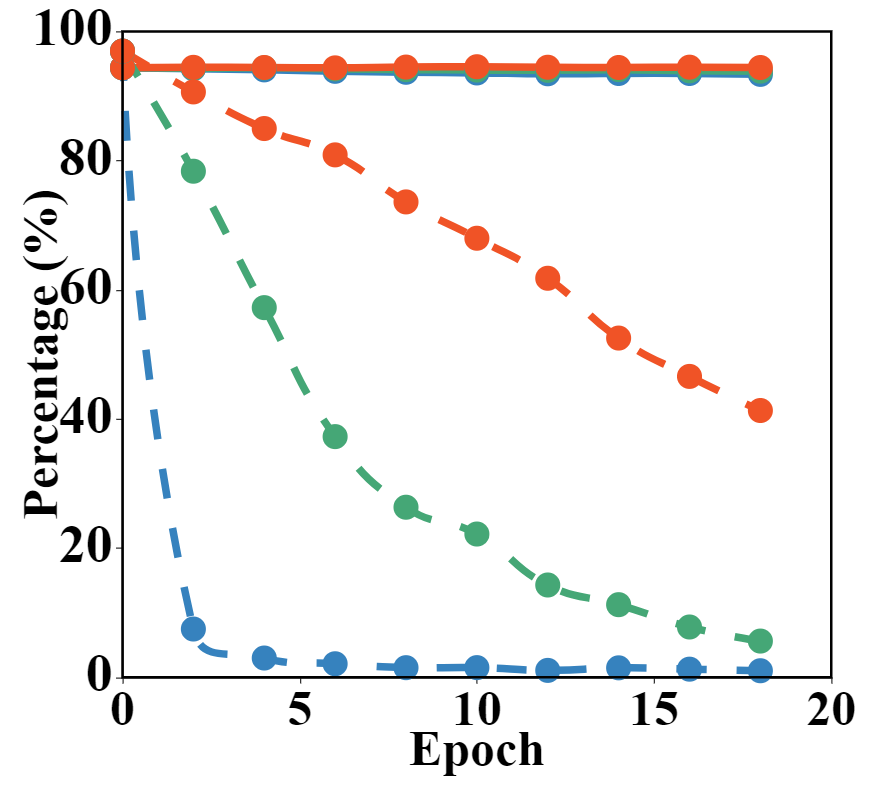}
    \caption{SIG}
\end{subfigure}
\begin{subfigure}{0.15\textwidth}
\centering
    \includegraphics[width=0.99\linewidth]{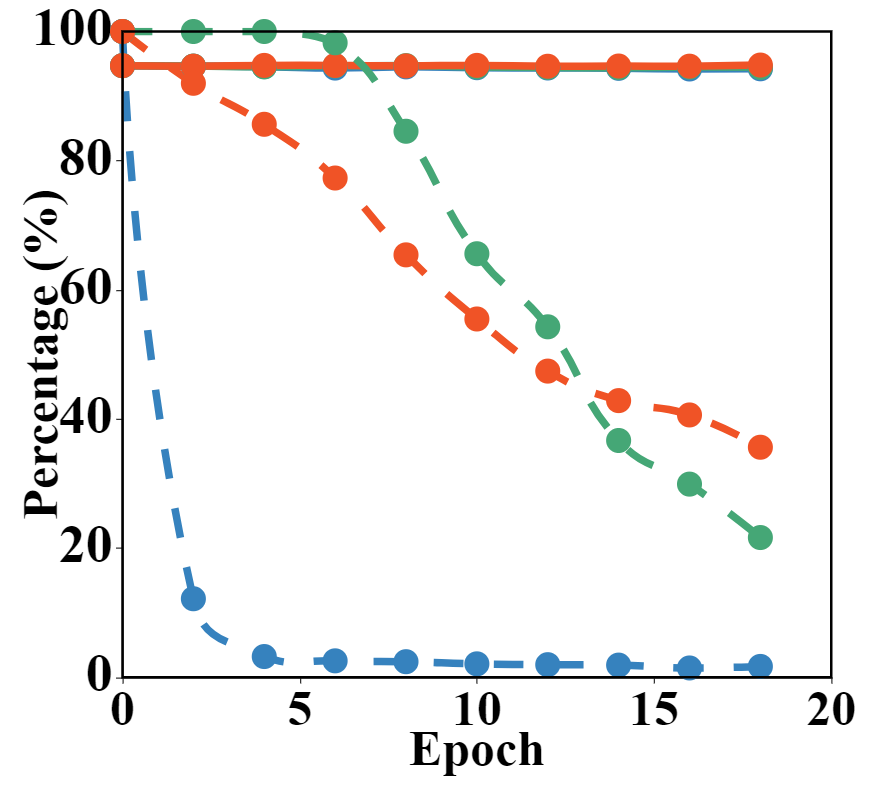}
    \caption{TrojanNN}
\end{subfigure}
\begin{subfigure}{0.05\textwidth}
\centering
    \includegraphics[width=0.99\linewidth]{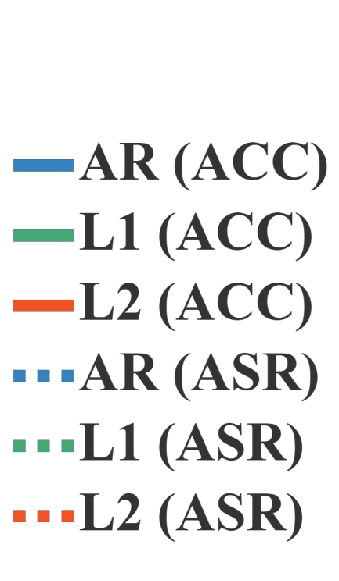}
\end{subfigure}
\caption{The performance of \sysname with different regularization items ($L_1$, $L_2$, and $AR$) on SVHN.}
\label{regularization_svhn}
\end{figure*}

\begin{figure*}[!h]
\centering
\begin{subfigure}{0.15\textwidth}
\centering
    \includegraphics[width=0.99\linewidth]{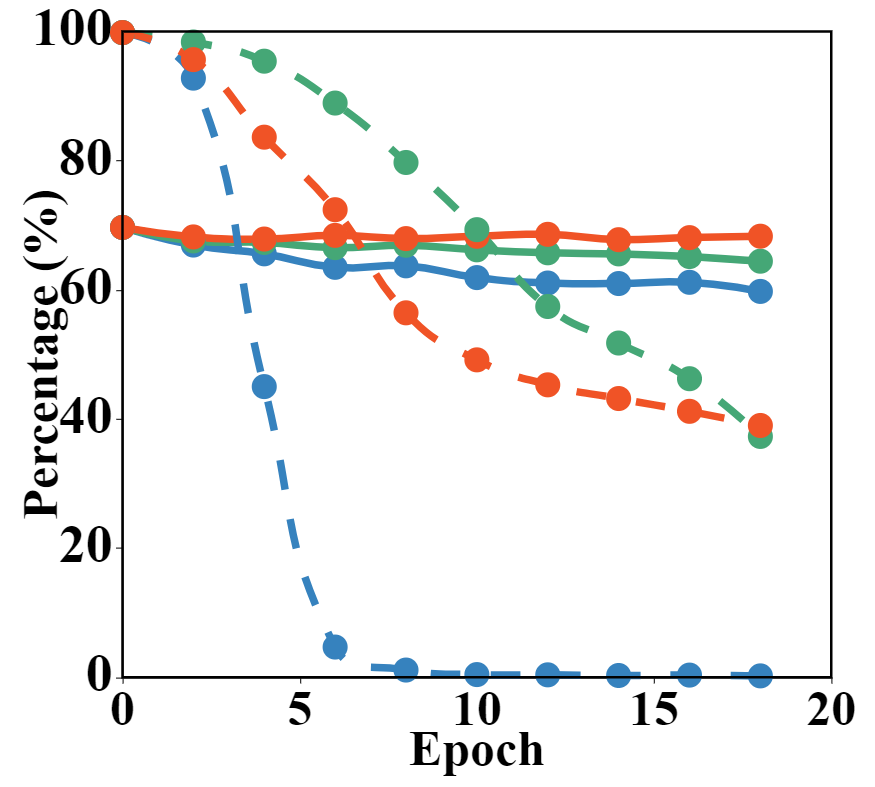}
    \caption{BadNet}
\end{subfigure}%
\begin{subfigure}{0.15\textwidth}
\centering
    \includegraphics[width=0.99\linewidth]{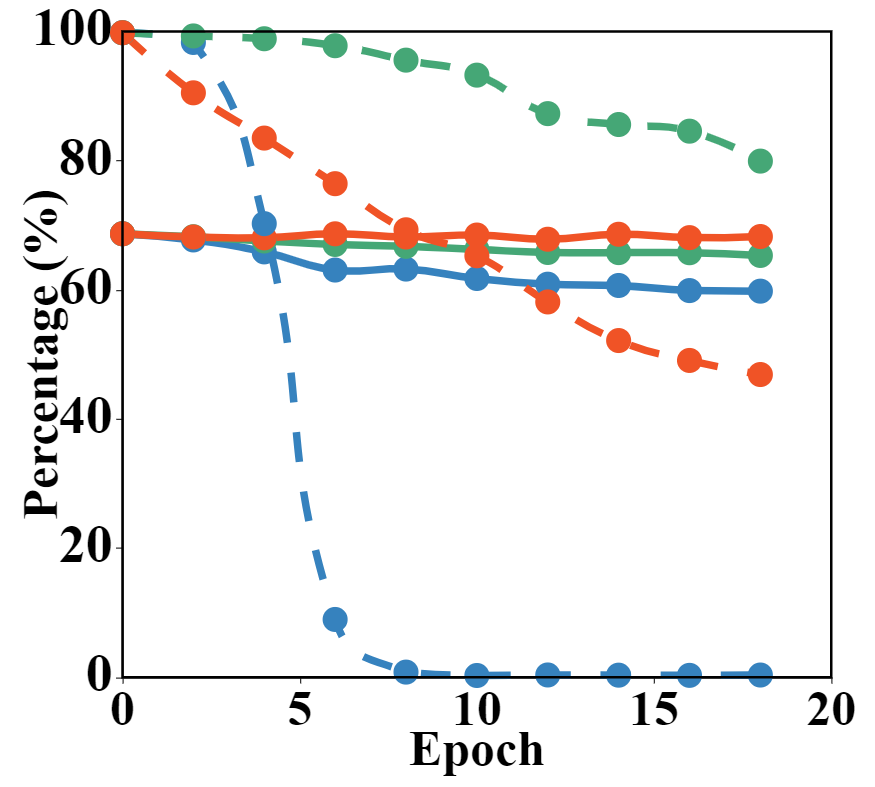}
    \caption{BA}
\end{subfigure}
\begin{subfigure}{0.15\textwidth}
\centering
    \includegraphics[width=0.99\linewidth]{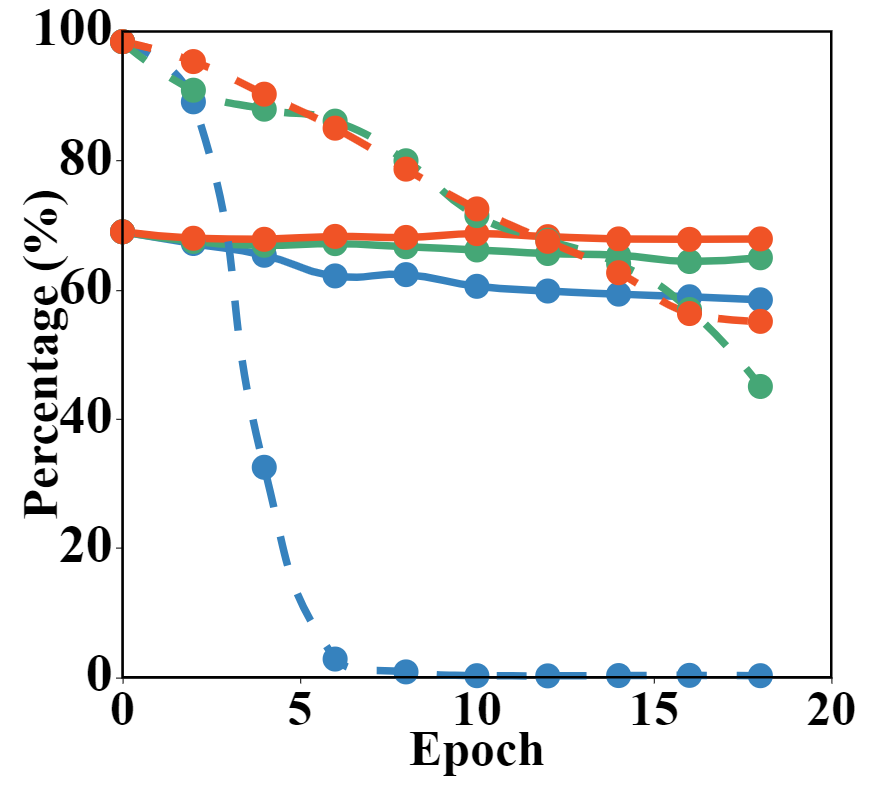}
    \caption{ETA}
\end{subfigure}
\begin{subfigure}{0.15\textwidth}
\centering
    \includegraphics[width=0.99\linewidth]{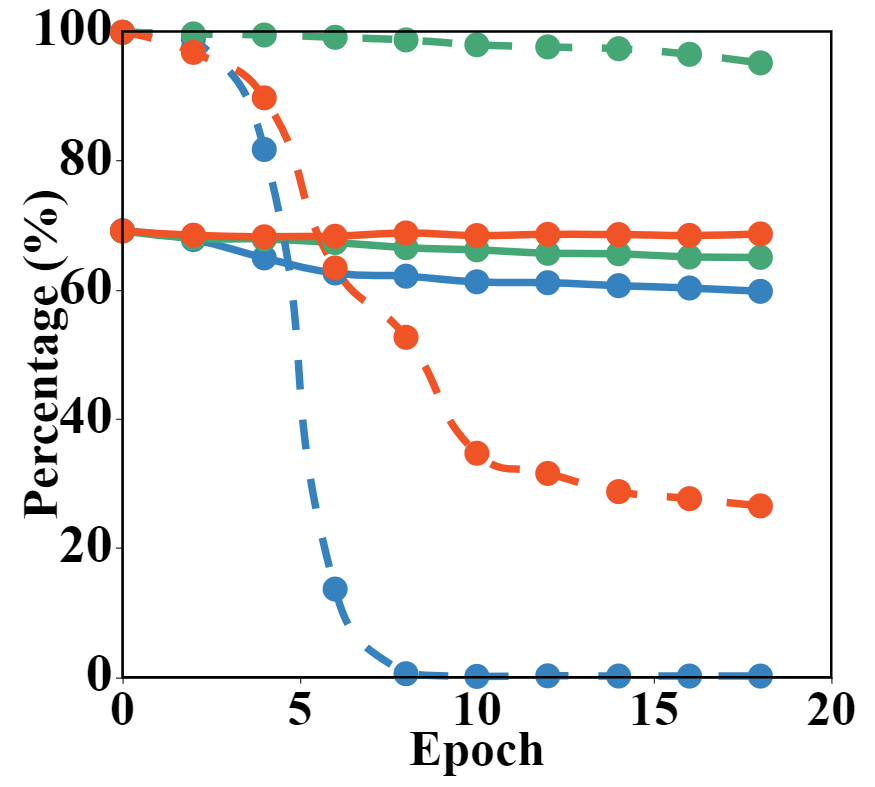}
    \caption{IA}
\end{subfigure}
\begin{subfigure}{0.15\textwidth}
\centering
    \includegraphics[width=0.99\linewidth]{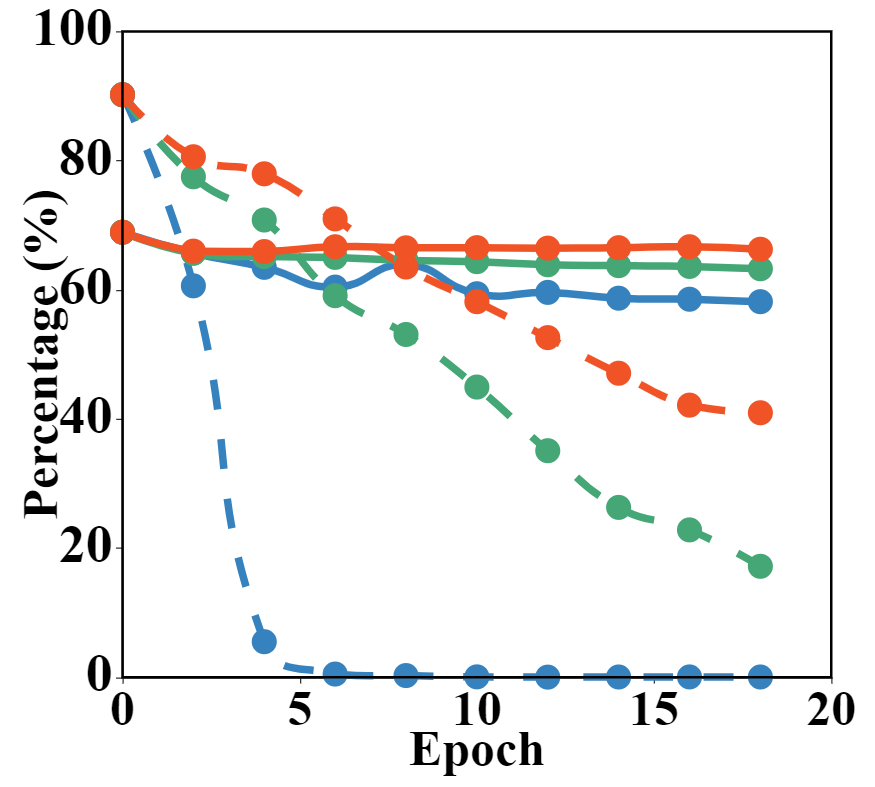}
    \caption{SIG}
\end{subfigure}
\begin{subfigure}{0.15\textwidth}
\centering
    \includegraphics[width=0.99\linewidth]{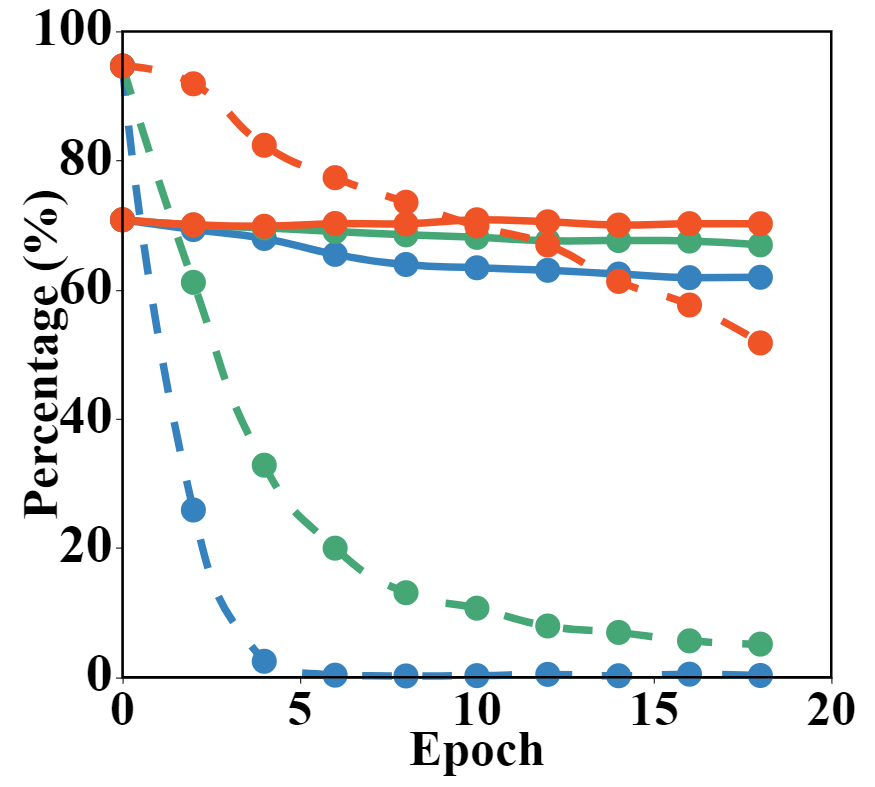}
    \caption{TrojanNN}
\end{subfigure}
\begin{subfigure}{0.05\textwidth}
\centering
    \includegraphics[width=0.99\linewidth]{images/legend.png}
\end{subfigure}
\caption{The performance of \sysname with different regularization items ($L_1$, $L_2$, and $AR$) on CIFAR-100.}
\label{regularization_cifar100}
\end{figure*}

\section{Experiment results in SVHN and CIFAR-100}
Here we report the experiment results on SVHN and CIFAR-100 as supplements.
Roughly speaking, we can obtain similar conclusions based on Table \ref{table_importance_comp_svhn}, Table \ref{table_importance_comp_cifar100}, Figure \ref{regularization_svhn}, Figure \ref{regularization_cifar100}, Figure \ref{data_ratio_svhn}, and Figure \ref{data_ratio_cifar100}.

\begin{figure*}[!h]
\centering
\begin{subfigure}{0.16\textwidth}
\centering
    \includegraphics[width=0.99\linewidth]{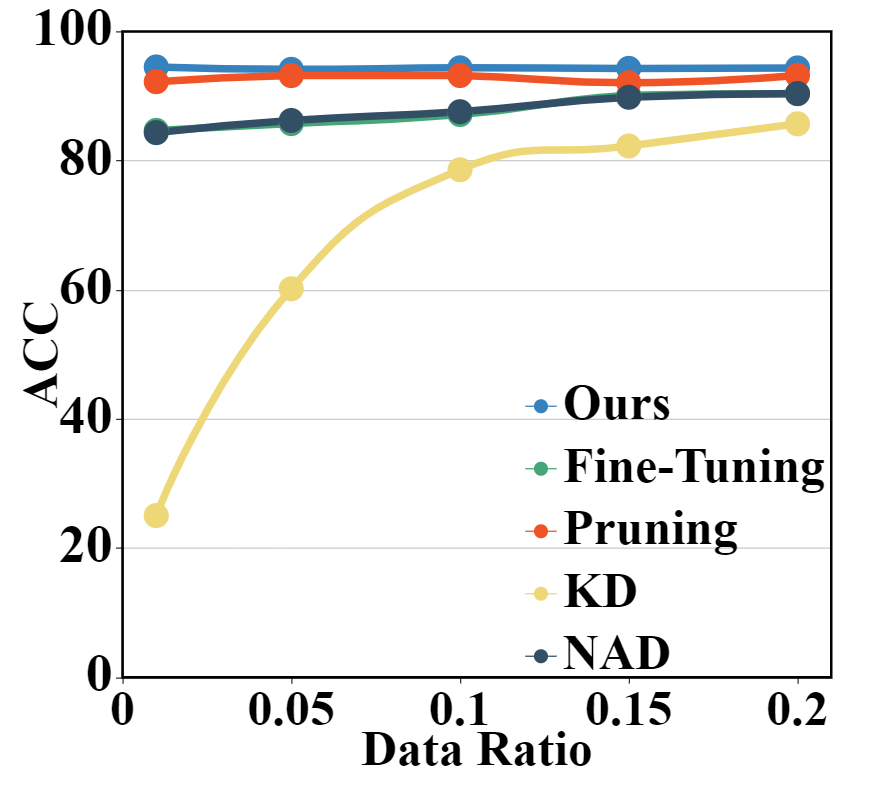}
    \caption{BadNet}
\end{subfigure}%
\begin{subfigure}{0.16\textwidth}
\centering
    \includegraphics[width=0.99\linewidth]{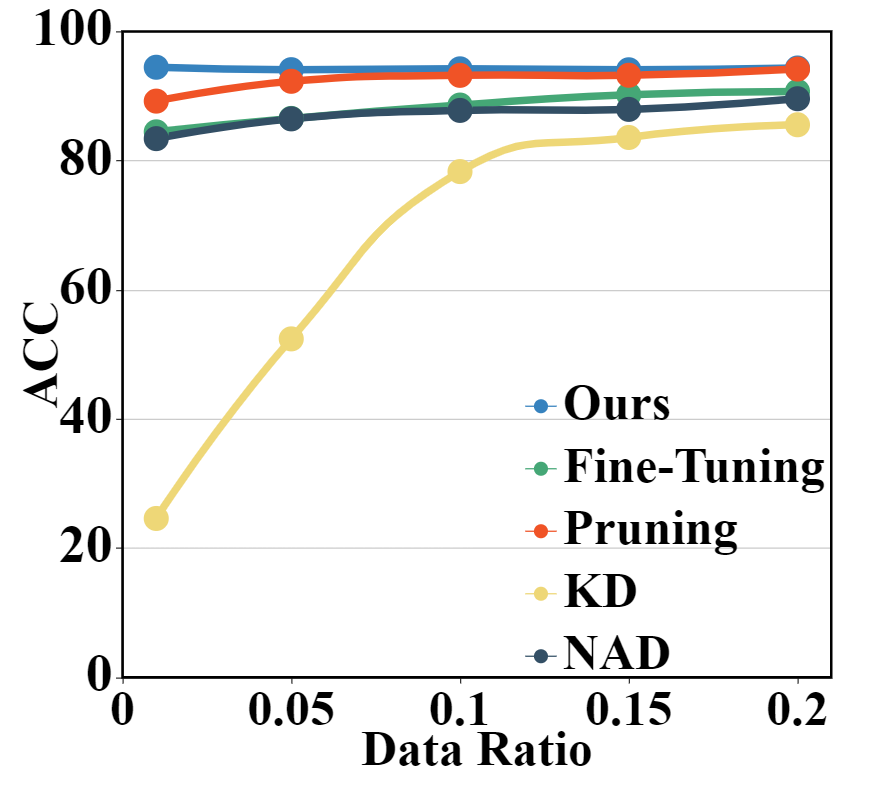}
    \caption{BA}
\end{subfigure}
\begin{subfigure}{0.16\textwidth}
\centering
    \includegraphics[width=0.99\linewidth]{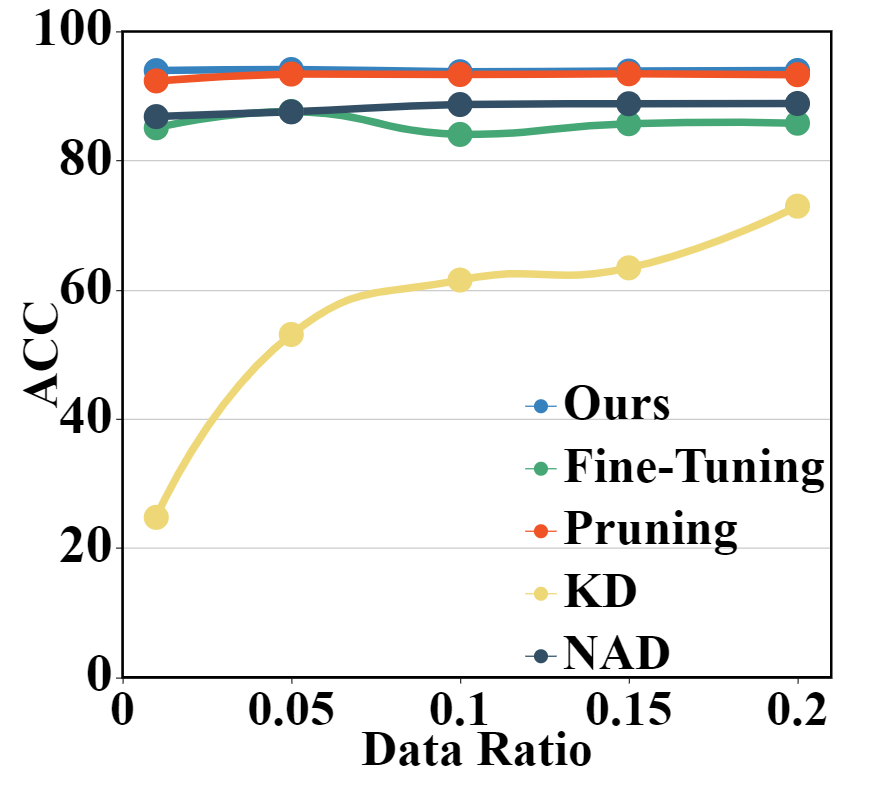}
    \caption{ETA}
\end{subfigure}
\begin{subfigure}{0.16\textwidth}
\centering
    \includegraphics[width=0.99\linewidth]{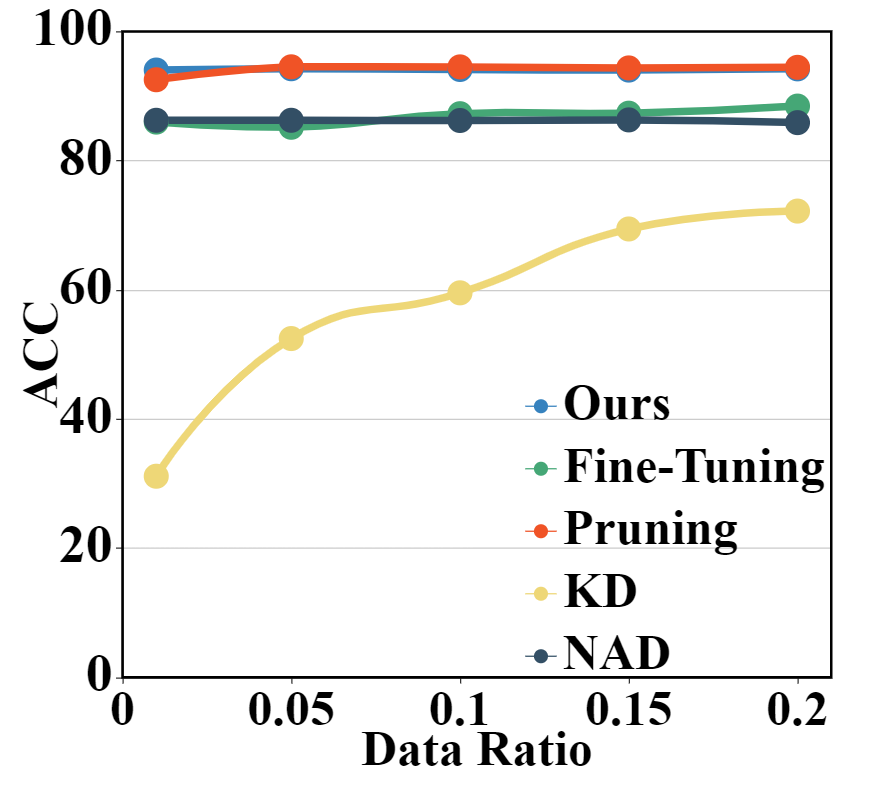}
    \caption{IA}
\end{subfigure}
\begin{subfigure}{0.16\textwidth}
\centering
    \includegraphics[width=0.99\linewidth]{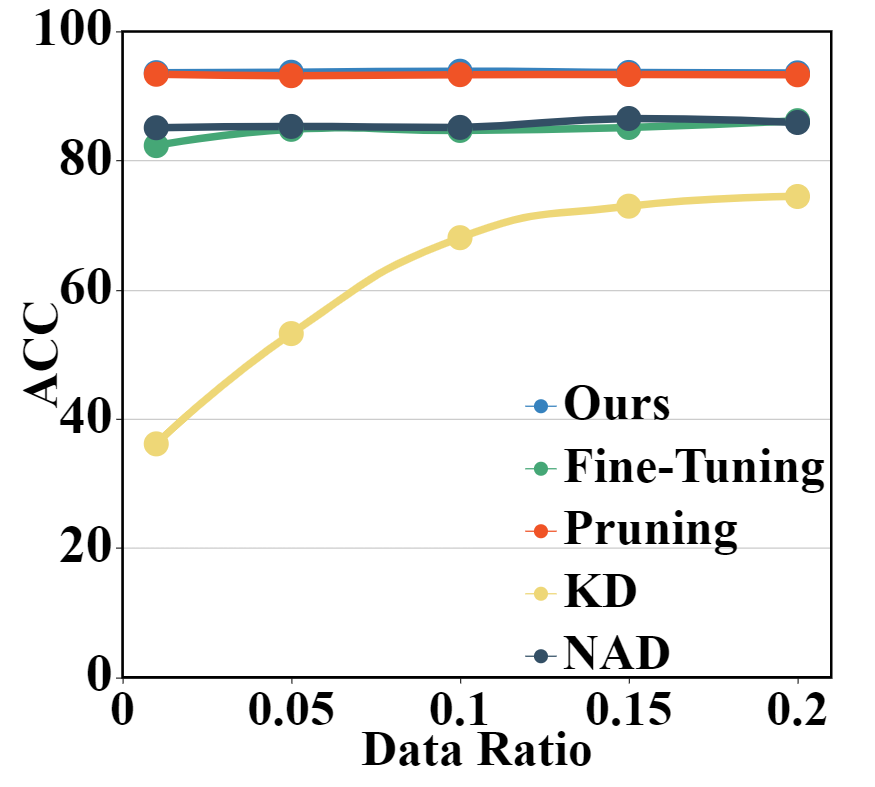}
    \caption{SIG}
\end{subfigure}
\begin{subfigure}{0.16\textwidth}
\centering
    \includegraphics[width=0.99\linewidth]{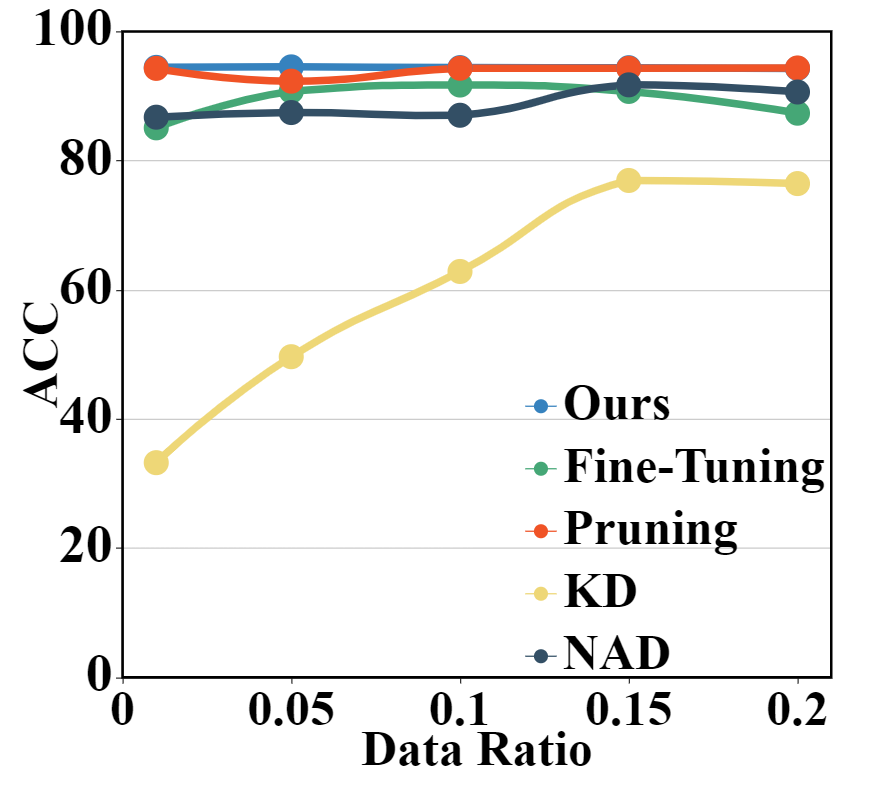}
    \caption{TrojanNN}
\end{subfigure}
\begin{subfigure}{0.16\textwidth}
\centering
    \includegraphics[width=0.99\linewidth]{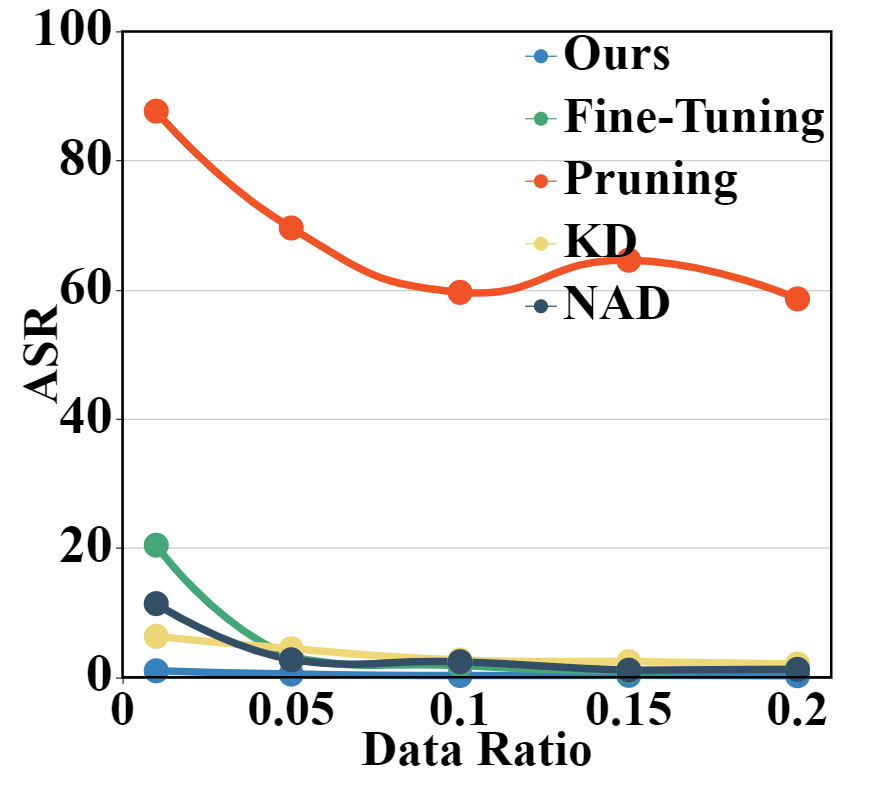}
    \caption{BadNet}
\end{subfigure}%
\begin{subfigure}{0.16\textwidth}
\centering
    \includegraphics[width=0.99\linewidth]{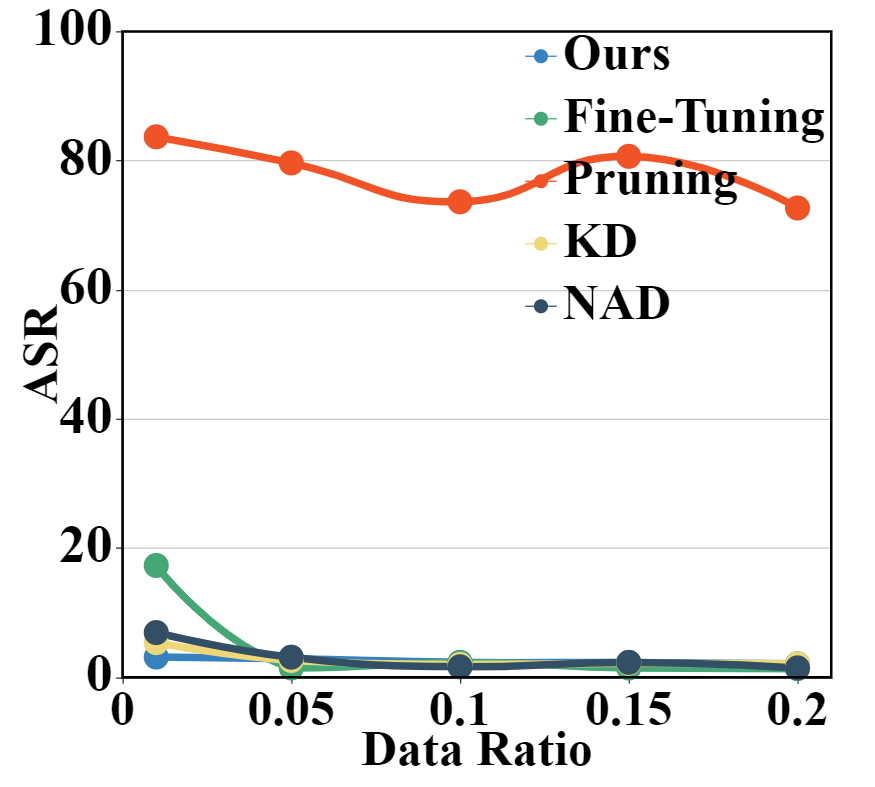}
    \caption{BA}
\end{subfigure}
\begin{subfigure}{0.16\textwidth}
\centering
    \includegraphics[width=0.99\linewidth]{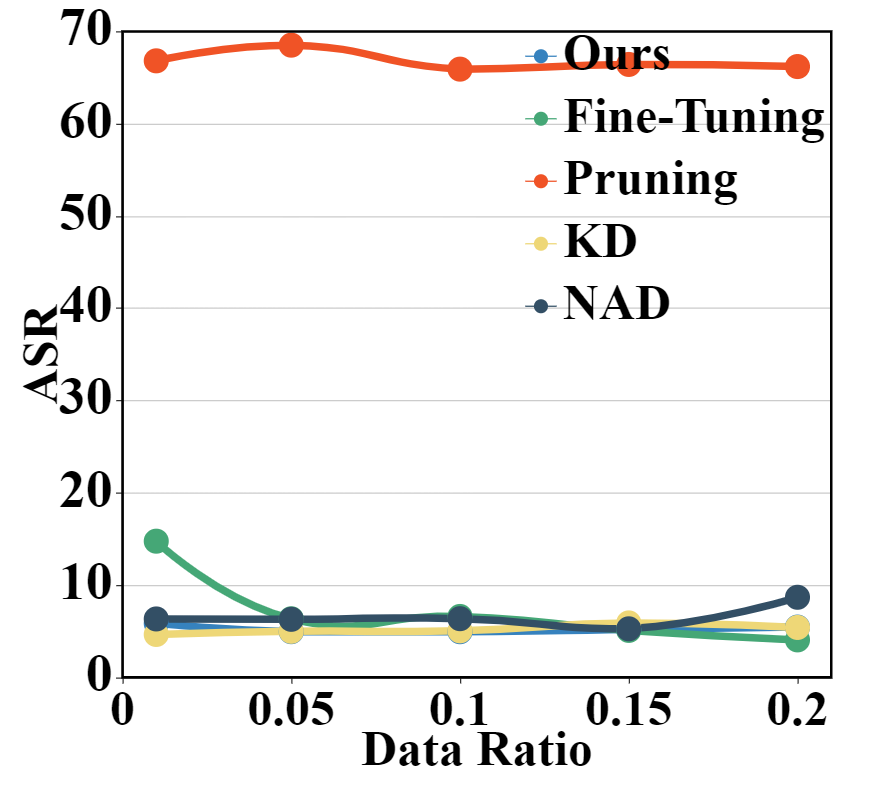}
    \caption{ETA}
\end{subfigure}
\begin{subfigure}{0.16\textwidth}
\centering
    \includegraphics[width=0.99\linewidth]{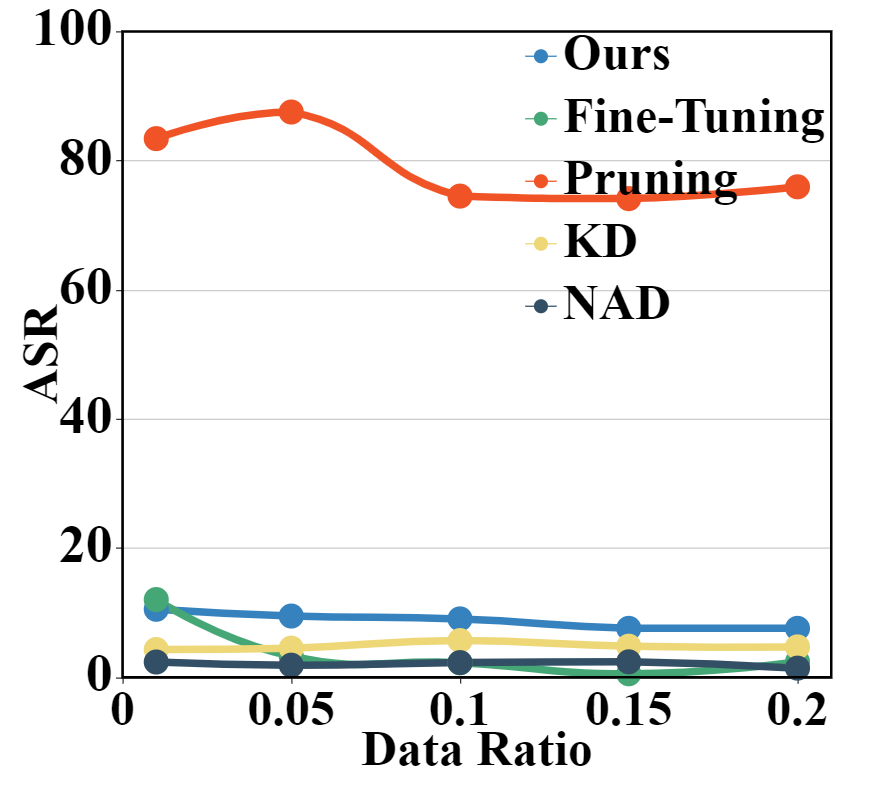}
    \caption{IA}
\end{subfigure}
\begin{subfigure}{0.16\textwidth}
\centering
    \includegraphics[width=0.99\linewidth]{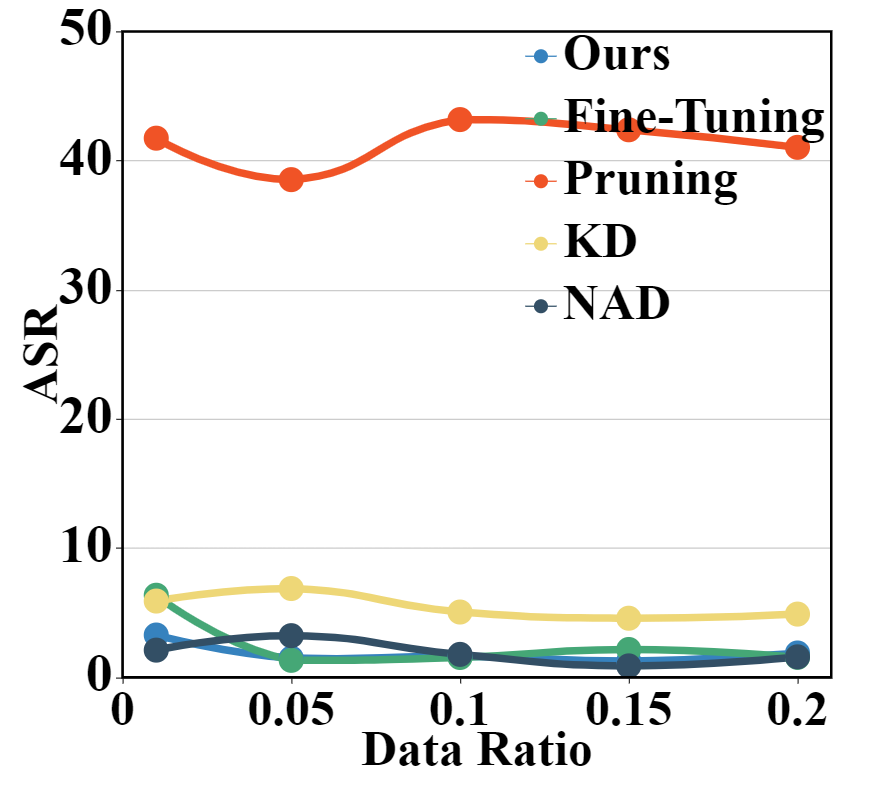}
    \caption{SIG}
\end{subfigure}
\begin{subfigure}{0.16\textwidth}
\centering
    \includegraphics[width=0.99\linewidth]{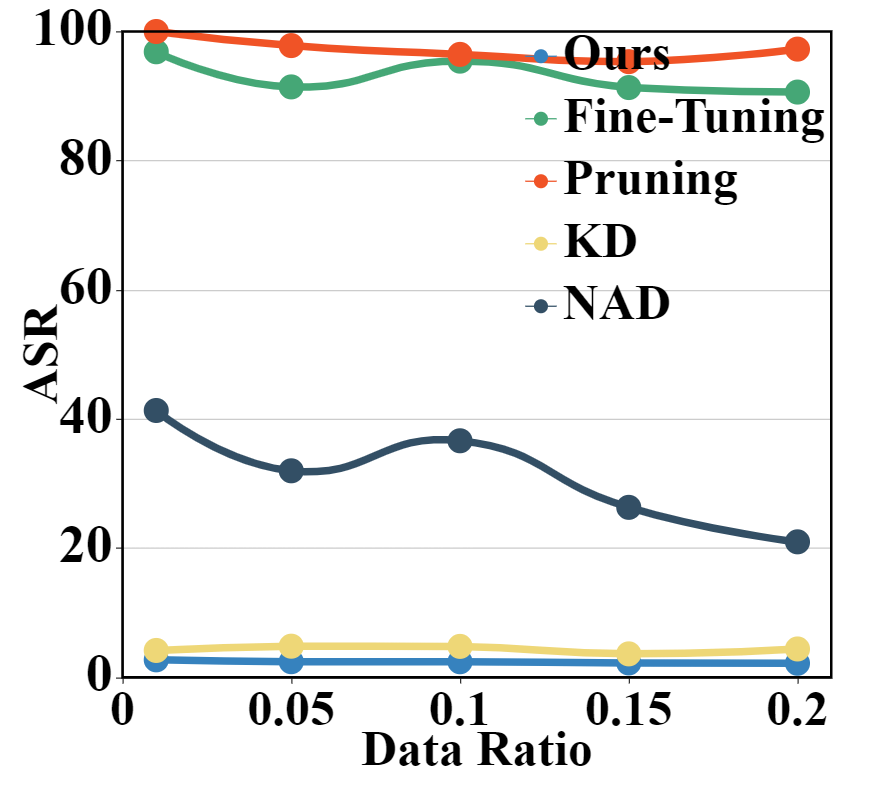}
    \caption{TrojanNN}
\end{subfigure}
\caption{The defense performance of five defense methods over different data ratio (0.01, 0.05, 0.1, 0.15, 0.2) in SVHN.}
\label{data_ratio_svhn}
\end{figure*}

\begin{figure*}[!h]
\centering
\begin{subfigure}{0.16\textwidth}
\centering
    \includegraphics[width=0.99\linewidth]{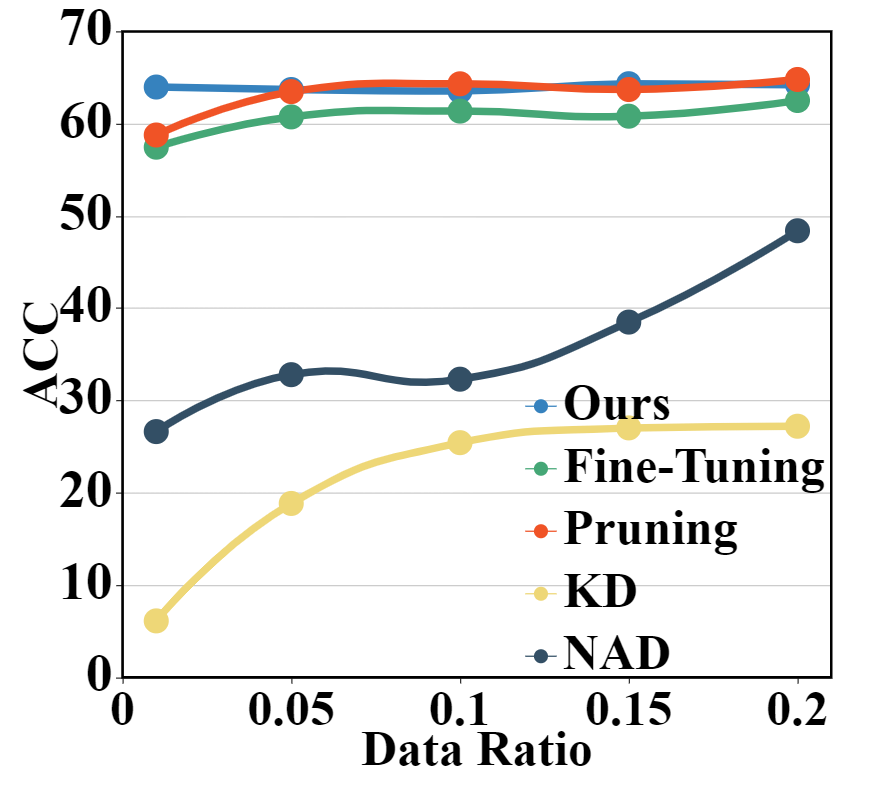}
    \caption{BadNet}
\end{subfigure}%
\begin{subfigure}{0.16\textwidth}
\centering
    \includegraphics[width=0.99\linewidth]{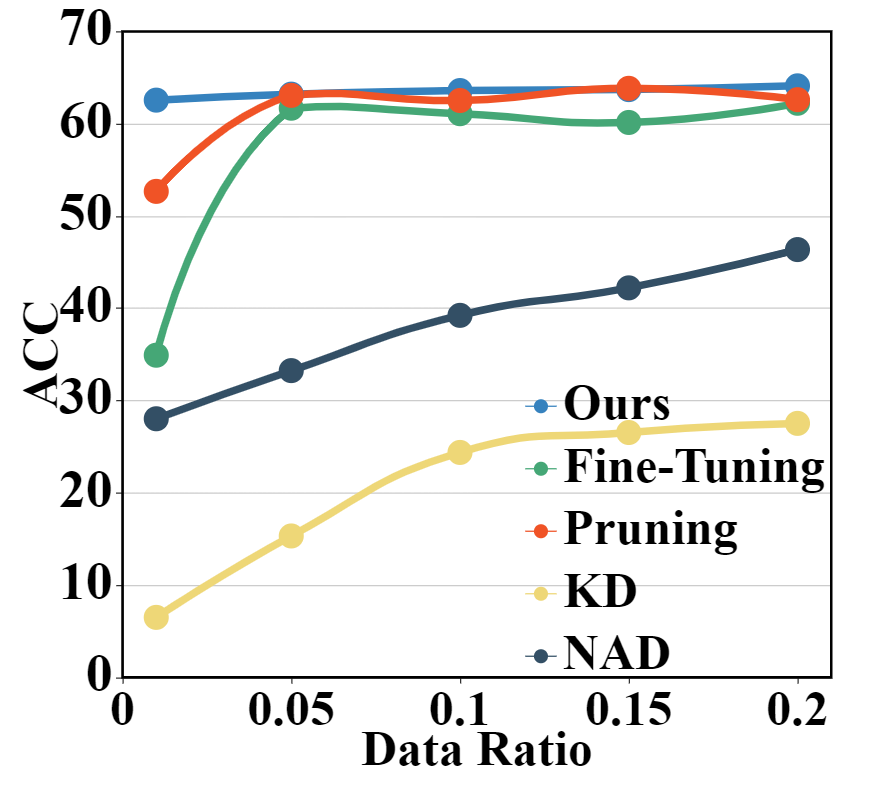}
    \caption{BA}
\end{subfigure}
\begin{subfigure}{0.16\textwidth}
\centering
    \includegraphics[width=0.99\linewidth]{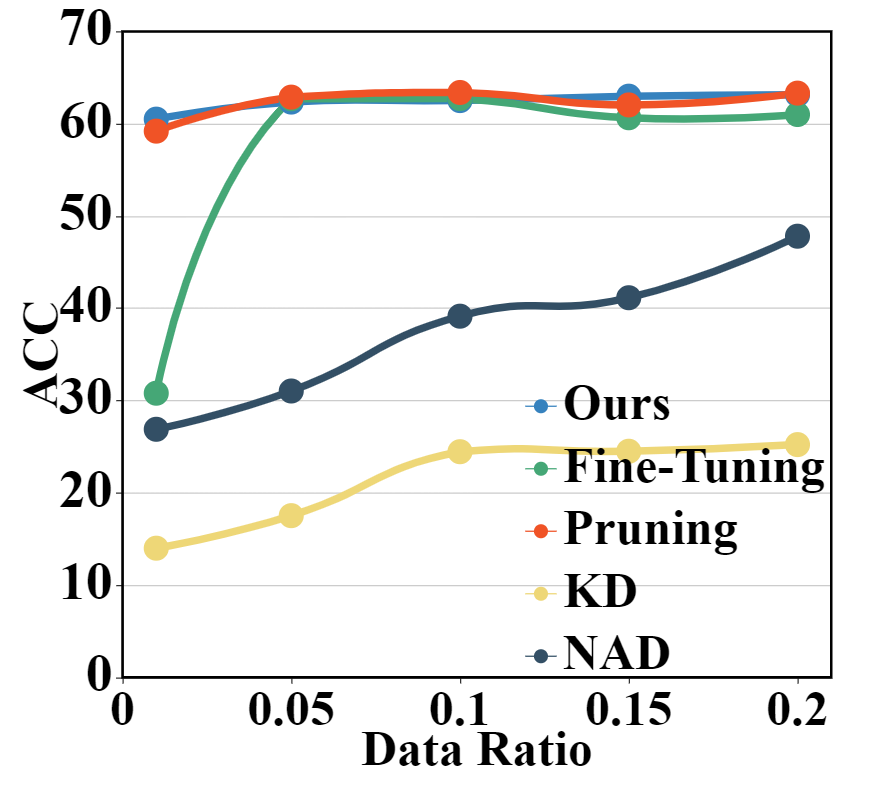}
    \caption{ETA}
\end{subfigure}
\begin{subfigure}{0.16\textwidth}
\centering
    \includegraphics[width=0.99\linewidth]{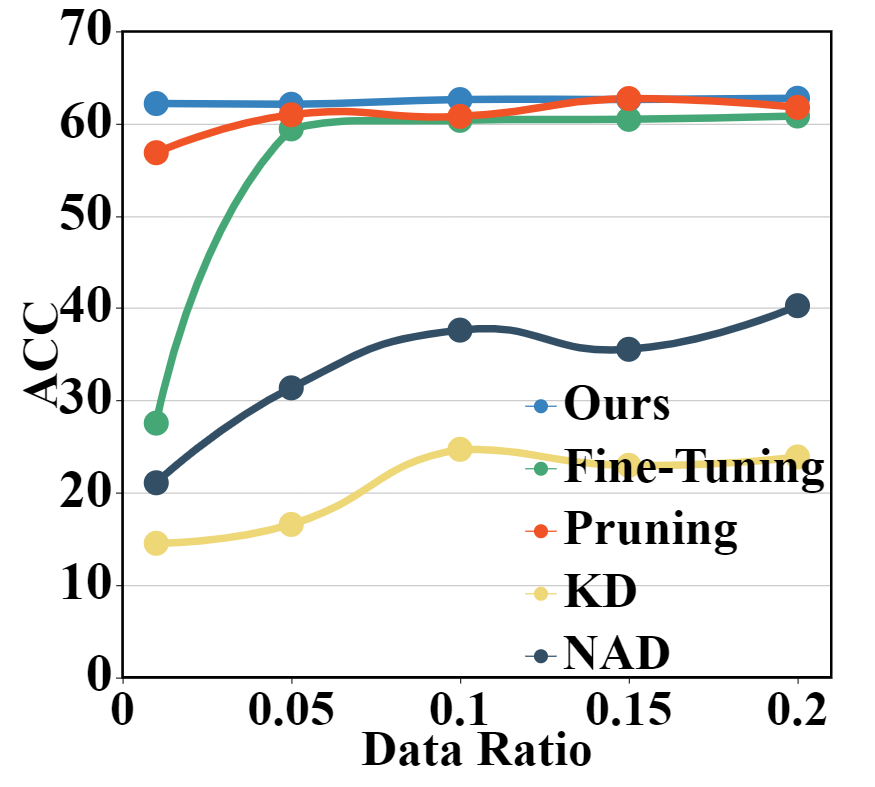}
    \caption{IA}
\end{subfigure}
\begin{subfigure}{0.16\textwidth}
\centering
    \includegraphics[width=0.99\linewidth]{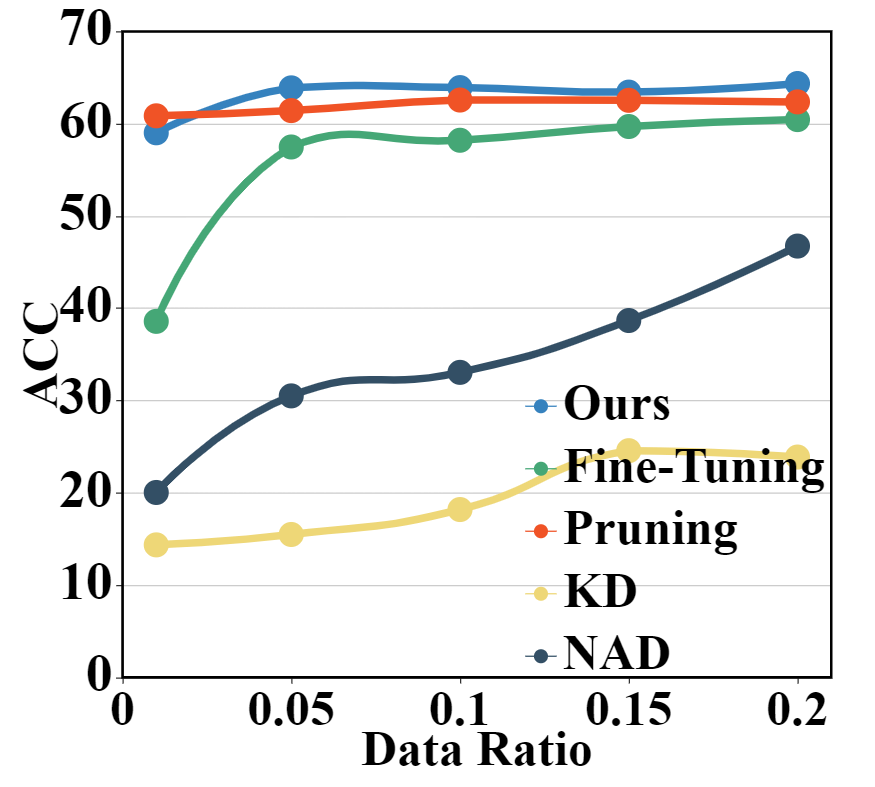}
    \caption{SIG}
\end{subfigure}
\begin{subfigure}{0.16\textwidth}
\centering
    \includegraphics[width=0.99\linewidth]{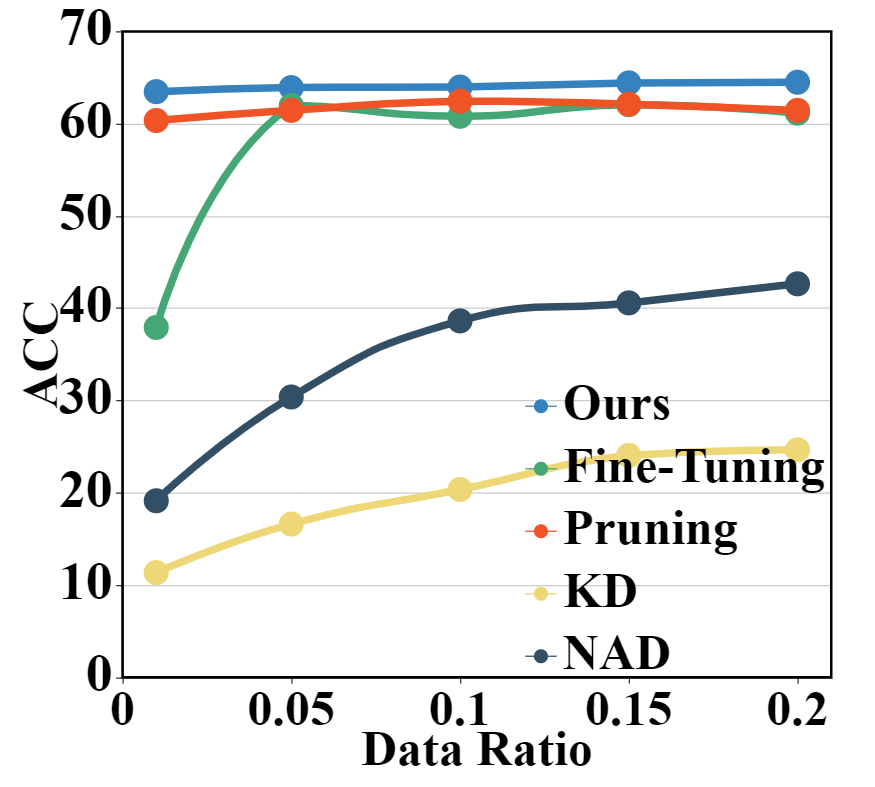}
    \caption{TrojanNN}
\end{subfigure}
\begin{subfigure}{0.16\textwidth}
\centering
    \includegraphics[width=0.99\linewidth]{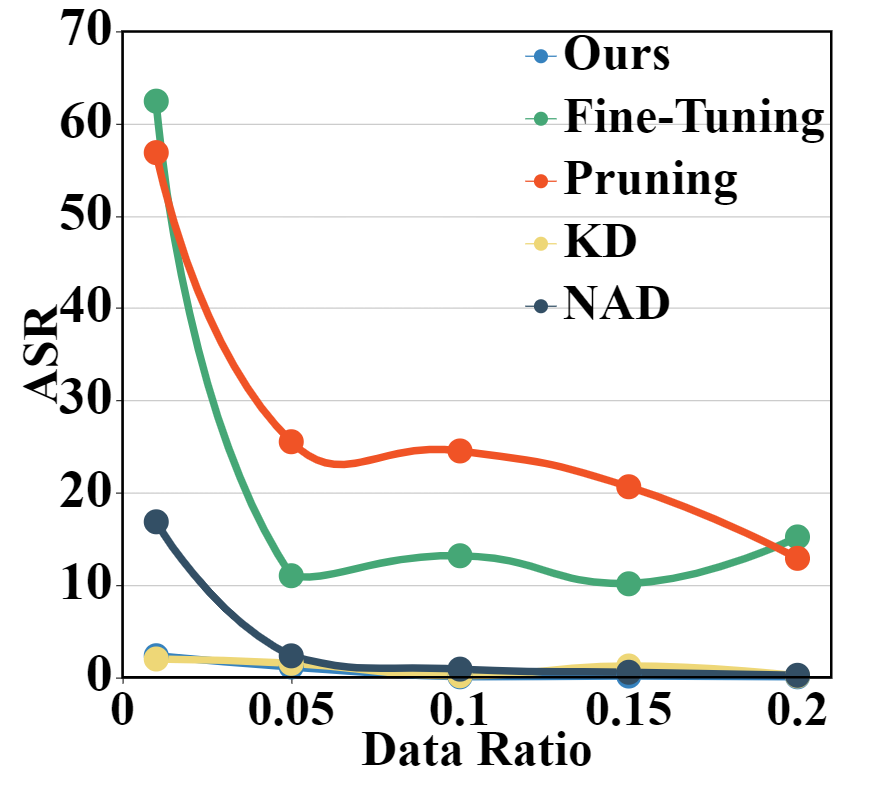}
    \caption{BadNet}
\end{subfigure}%
\begin{subfigure}{0.16\textwidth}
\centering
    \includegraphics[width=0.99\linewidth]{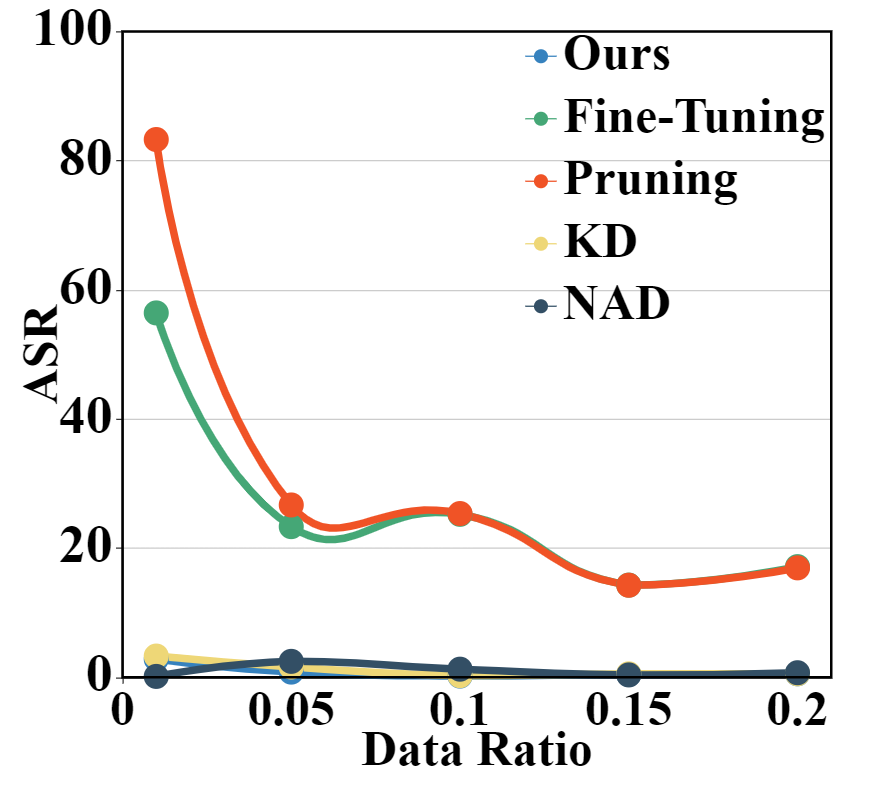}
    \caption{BA}
\end{subfigure}
\begin{subfigure}{0.16\textwidth}
\centering
    \includegraphics[width=0.99\linewidth]{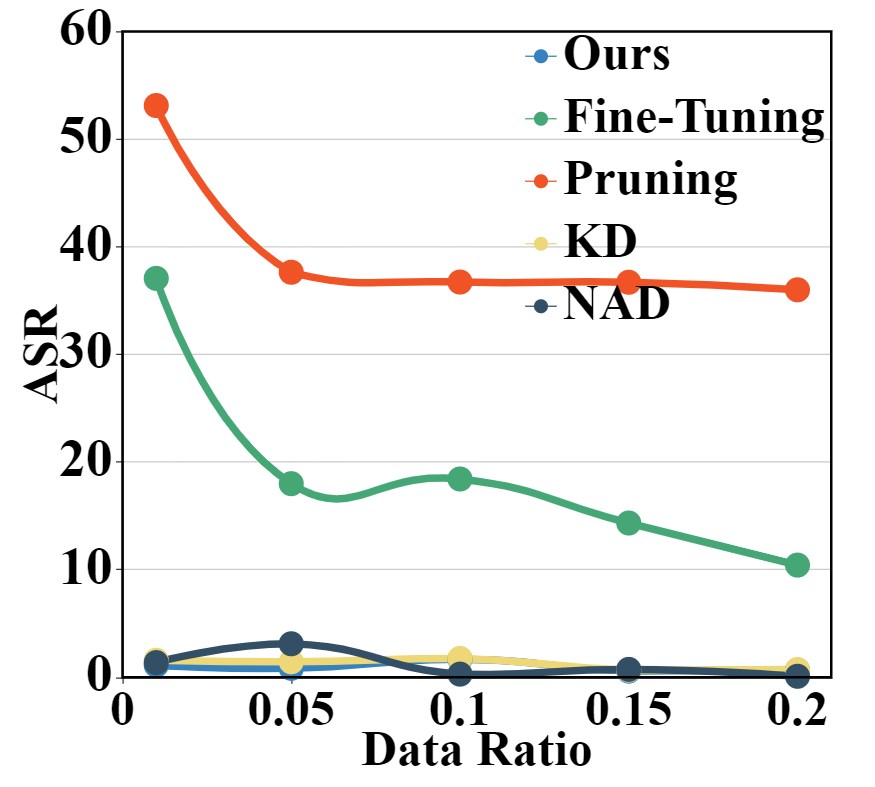}
    \caption{ETA}
\end{subfigure}
\begin{subfigure}{0.16\textwidth}
\centering
    \includegraphics[width=0.99\linewidth]{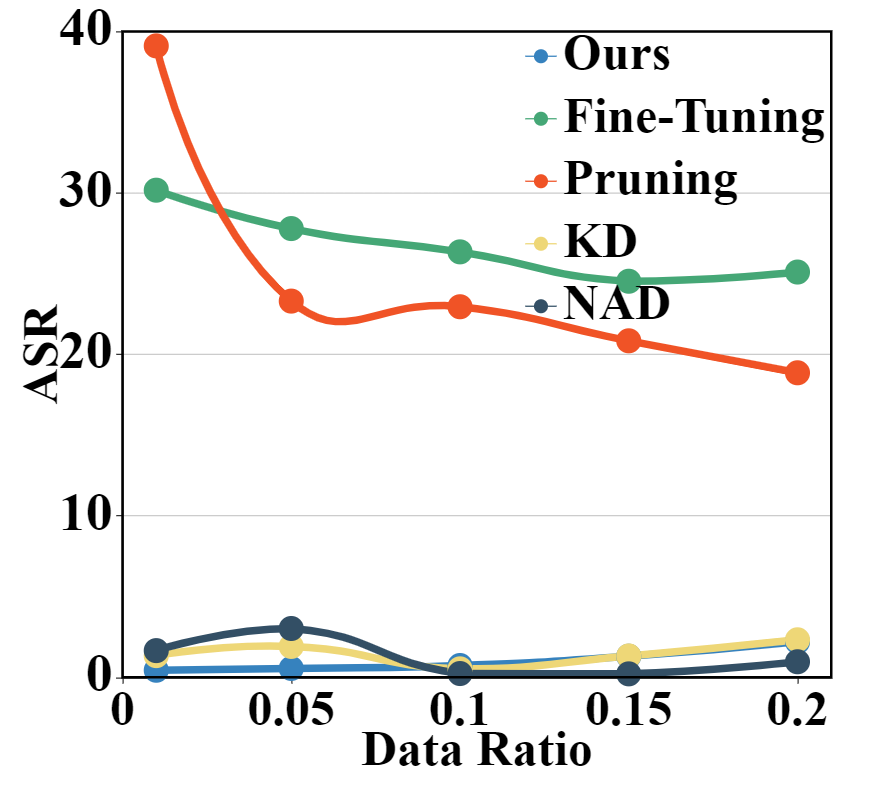}
    \caption{IA}
\end{subfigure}
\begin{subfigure}{0.16\textwidth}
\centering
    \includegraphics[width=0.99\linewidth]{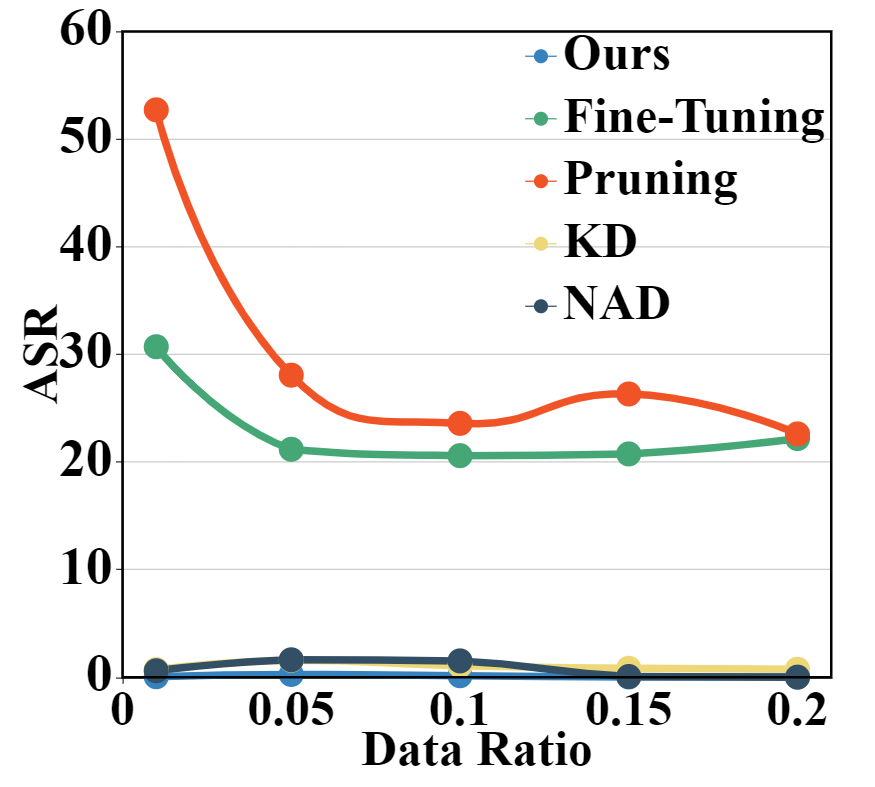}
    \caption{SIG}
\end{subfigure}
\begin{subfigure}{0.16\textwidth}
\centering
    \includegraphics[width=0.99\linewidth]{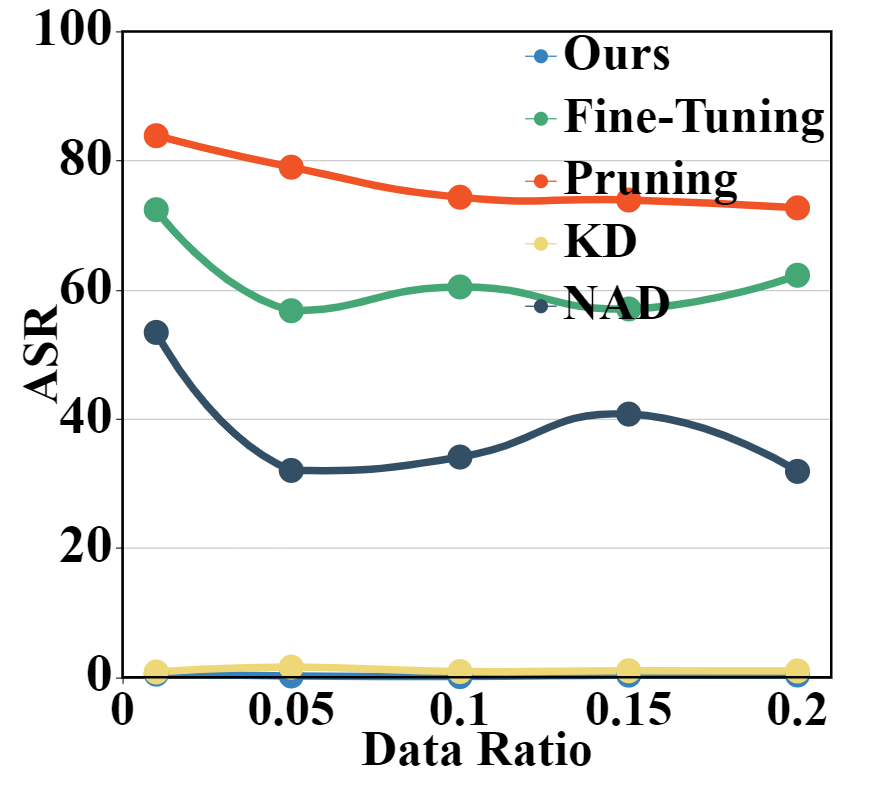}
    \caption{TrojanNN}
\end{subfigure}
\caption{The defense performance of five defense methods over different data ratio (0.01, 0.05, 0.1, 0.15, 0.2) in CIFAR-100.}
\label{data_ratio_cifar100}
\end{figure*}
